# Supplementary material for: Adaptive Regret for Control of Time-Varying Dynamics
Source: arXiv:2007.04393 source file (2022-02-12)
Supplement: Supplementary file 1 [file experiments.tex]

\section{Experimental Details}\label{sec:experiments_appendix}

\subsection{General Experimental Details}

\paragraph{Baseline Learner and Comparator(s).}As our baseline learner, we use the GPC algorithm described in \cite{agarwal2019logarithmic} and follow the implementation from TigerControl\footnote{\href{url}{https://github.com/MinRegret/TigerControl}}. We compare our performance to GPC and to the linear controller LQR which acts according to the algebraic Ricatti equation computed at the start of the experiment. For section \ref{sec:exp_pendulum}, we also compare against iLQR.

\paragraph{Implementation Details.}For AdaGPC, we implement a modified efficient version of Algorithm \ref{alg:adaptive_control} (described in section \ref{sec:efficient}) using GPC as the baseline controller. The changes we make for experimental purposes are: (i) we play the expert with the greatest weight at the given timestep (rather than sample), (ii) we instantiate a new learner every $20$ timesteps (rather than every timestep), and (iii) we pad the liftetimes so that they are at least $100$ timesteps.

\subsection{Time-varying LDS Experiments} \label{sec:exp_lds}

We first confirm the practicality of our theoretical results by applying our algorithm to the control of linear dynamical systems. The systems considered correspond to the settings in sections \ref{sec:fixed}, \ref{sec:switch_known} and \ref{sec:slow_known}, and are motivated by a physical mechanics application under alternating Gaussian i.i.d. and sinusoidal noise.

\paragraph{Experiment Setup.} We consider the control of fixed, switching and slowly changing linear dynamical systems. We measure performance via the quadratic cost function $c(x, u) = ||x||^2 + ||u||^2$. We average the results over $3$ runs and plot the corresponding mean performance and confidence intervals. 

\paragraph{General System Specification (+ physical interpretation).} We consider a system in which the state records the (one-dimensional) position and velocity of an object at time $t$ and the action corresponds to an input force, i.e. $x_t = \begin{bmatrix} q(t)  \\ \dot{q}(t) \end{bmatrix}$ and $u_t = \ddot{q}(t)$. Therefore, a system given by $A_\alpha = \begin{bmatrix} 1 & \alpha \\ 0 & 1 \end{bmatrix}$ and $B_\beta = \begin{bmatrix} 0  \\ \beta \end{bmatrix}$ represents a system in which the position is given by $q(t+1) = q(t) + \alpha \dot{q}(t)$ and its velocity is given by $\dot{q}(t+1) = \dot{q}(t) + \beta \ddot{q}(t)$. In particular, we consider the following three systems:

\begin{enumerate}[(a)]
\itemsep-0.3em
\item \textbf{Fixed system:}\label{fixed_system} we consider the canonical example of the double integrator system given by $A = \begin{bmatrix} 1 & 1 \\ 0 & 1 \end{bmatrix}$ and $B = \begin{bmatrix} 0  \\ 1\end{bmatrix}$ which models effect of a time-varying force input $u$ on a simple mass in one dimension.

    \item \textbf{Switching System:} \label{switching_system} we consider the system given by $A_1 = \begin{bmatrix} 1 & 0.5 \\ 0 & 1 \end{bmatrix}$ and $B_1 = \begin{bmatrix} 0  \\ 1.2 \end{bmatrix}$ for the first $T/2$ timesteps and which then switches to $A_2 = \begin{bmatrix} 1 & 1.5 \\ 0 & 1 \end{bmatrix}$ and $B_2 = \begin{bmatrix} 0  \\ 0.9 \end{bmatrix}$ for the rest of the run. The switch is marked by a dotted black line.

    \item \textbf{Time-variant system:} \label{changing_system} we consider the slowly changing system given by $A = \begin{bmatrix} 1 & 1 \\ 0 & 1 \end{bmatrix}$ and $B_t = \begin{bmatrix} 0  \\ {2 + \sin(2\pi t/T)}\end{bmatrix}$. This system is directly based on (\ref{fixed_system}), with the modification that the force changes (non-linearly) between being 1x and 2x active.
\end{enumerate}

\paragraph{I. Gaussian Noise.} For our first experiment, we simply consider the systems described above under i.i.d. Gaussian perturbations, i.e. $w_t \sim \mathcal{N}(0, 0.3^2)$.

\begin{figure}[H]
\centering
\subfigure{\includegraphics[width=60mm]{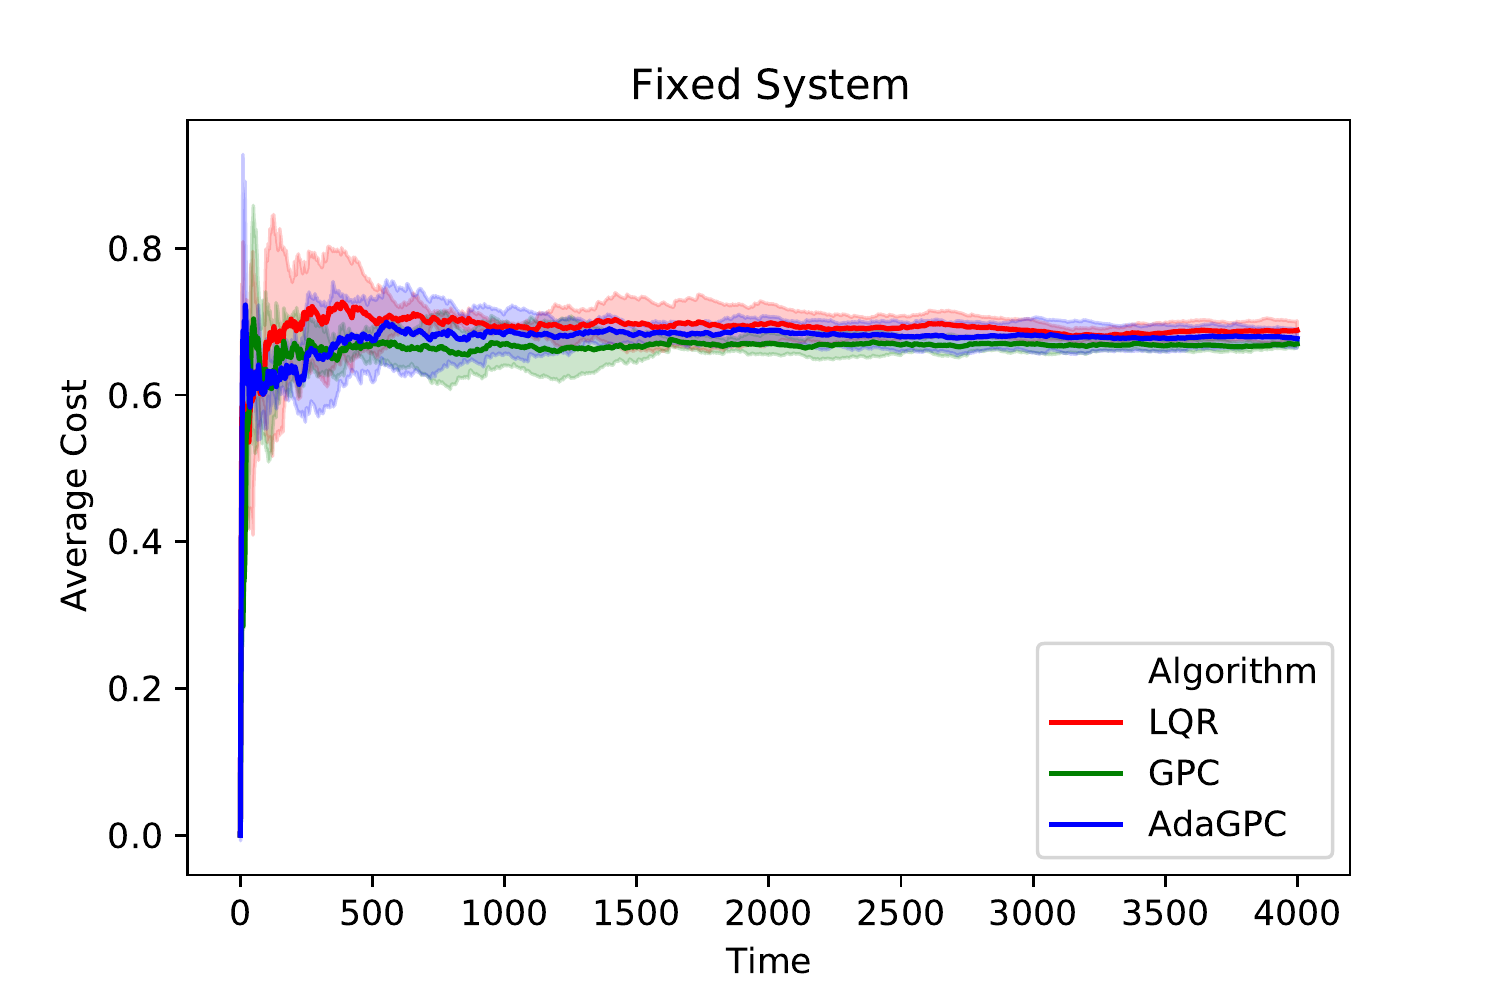}}
\subfigure{\includegraphics[width=60mm]{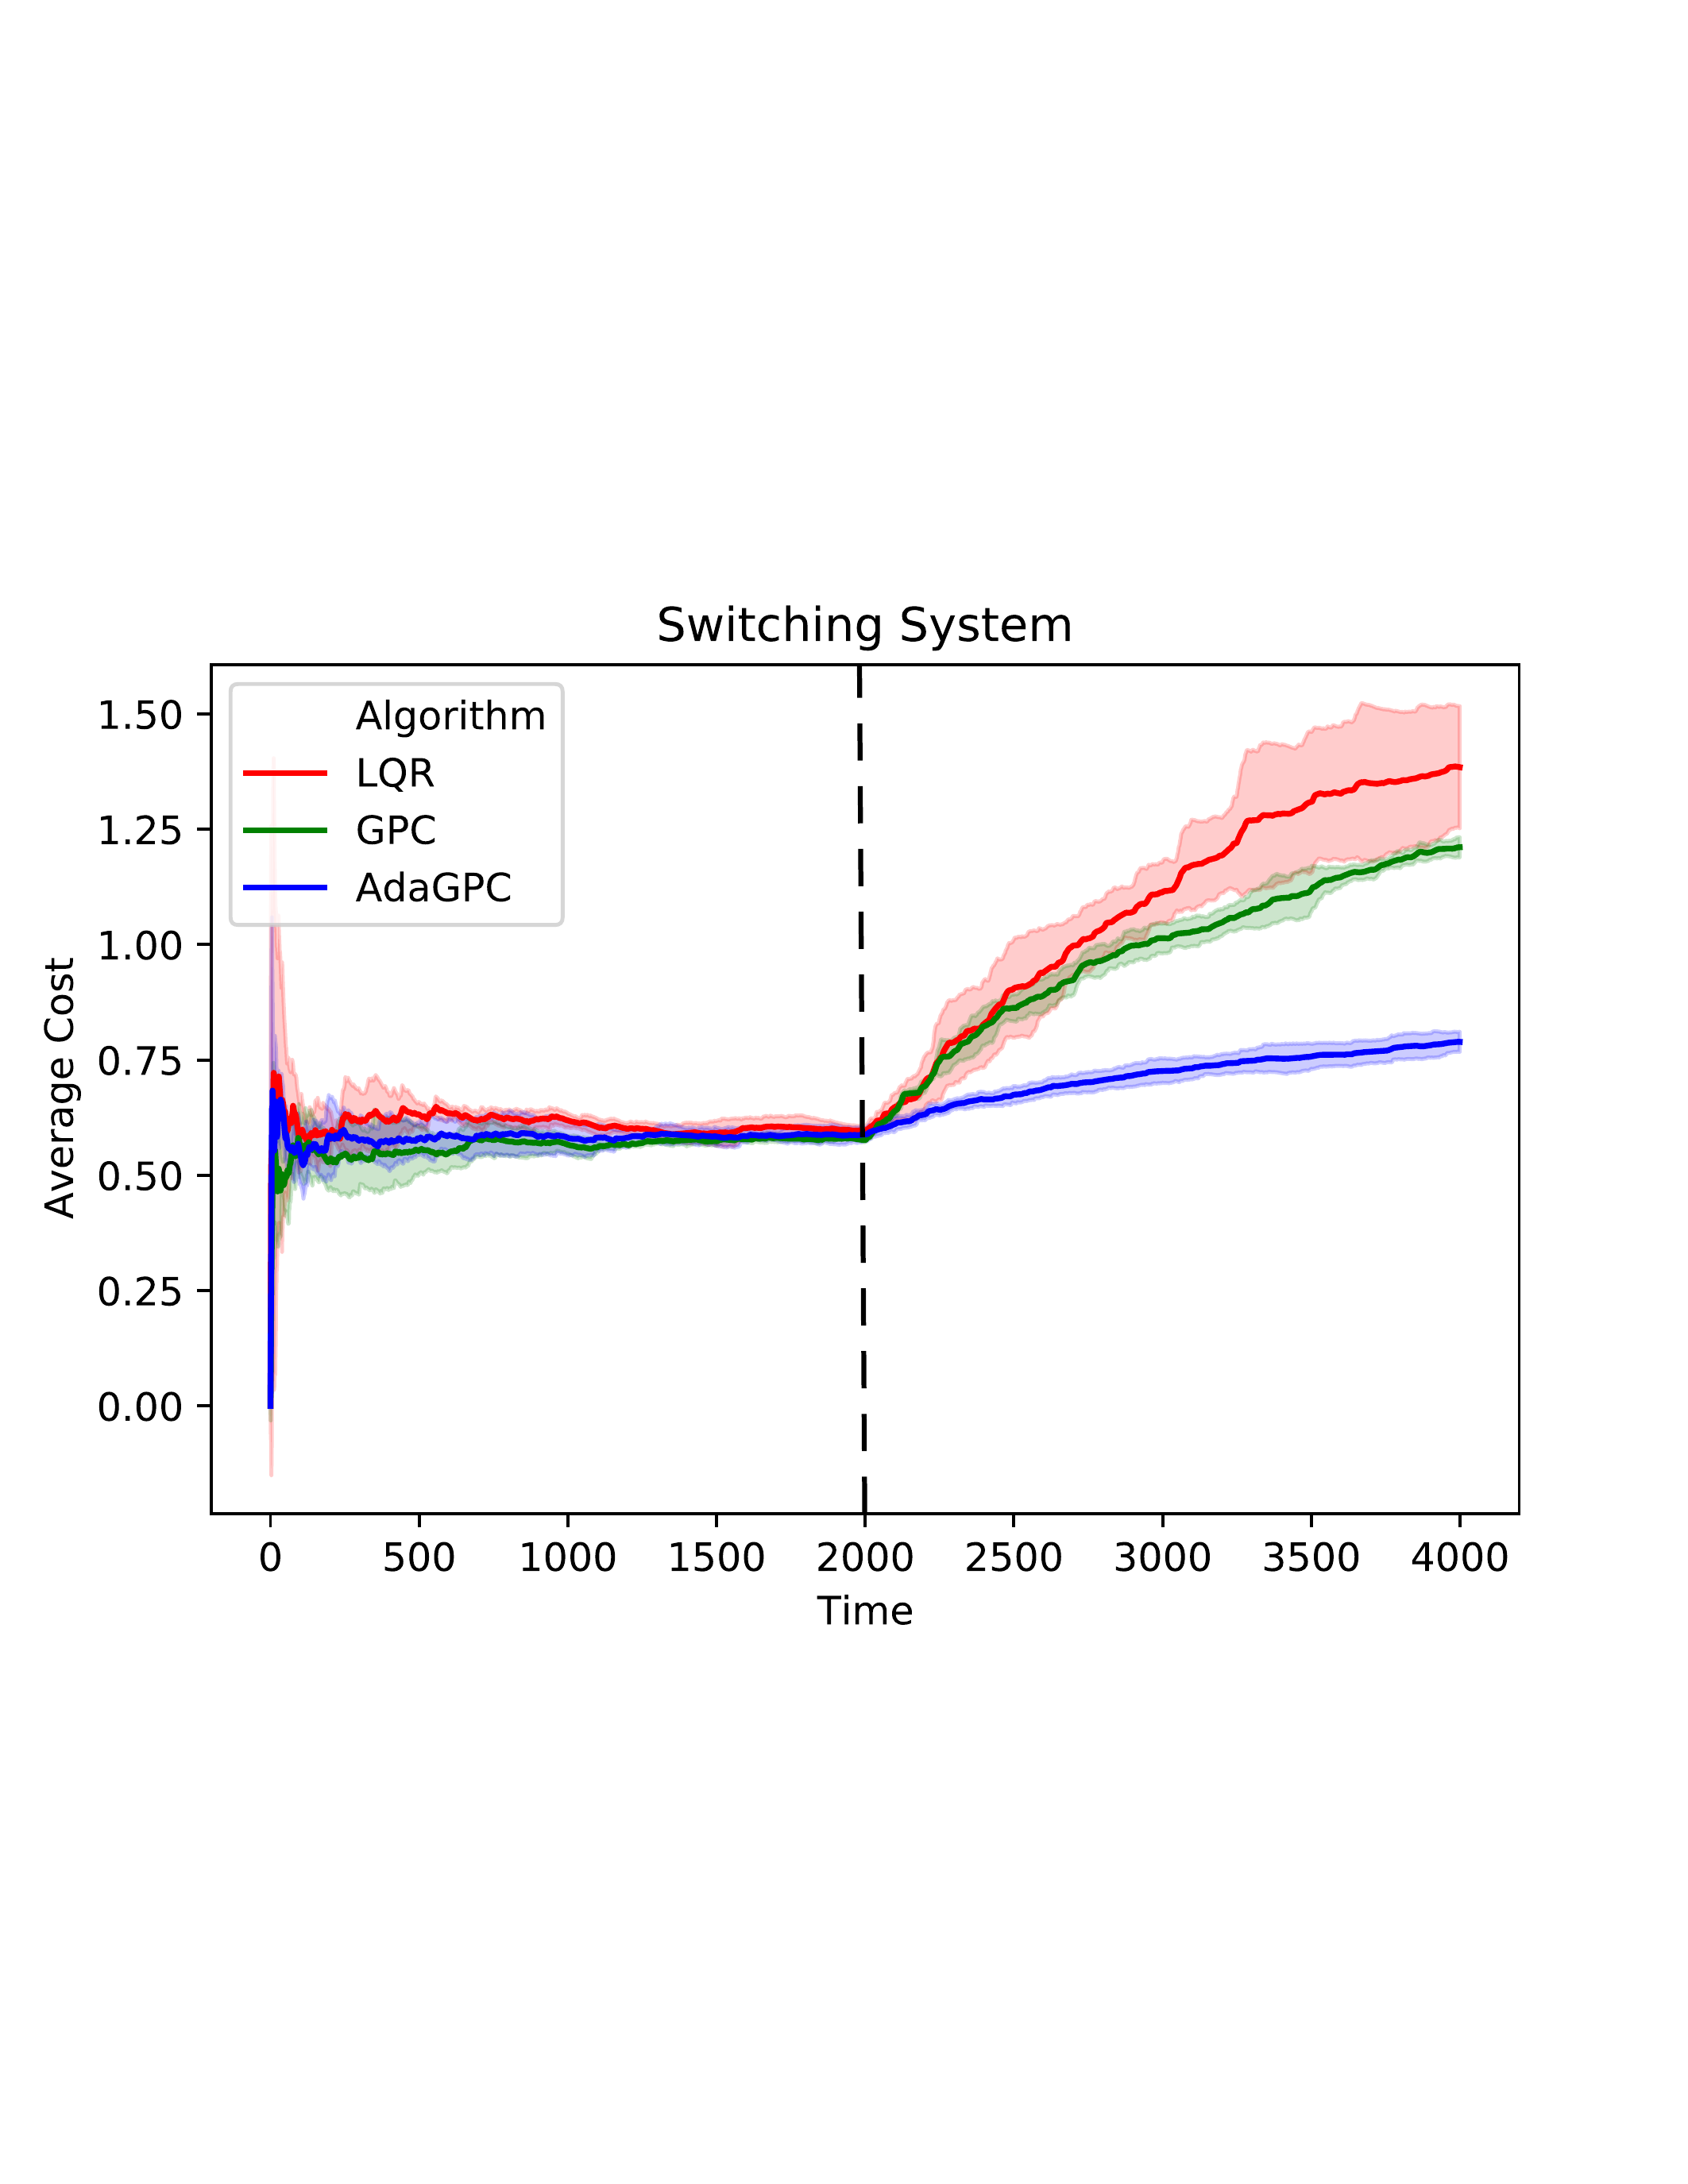}}
\subfigure{\includegraphics[width=60mm]{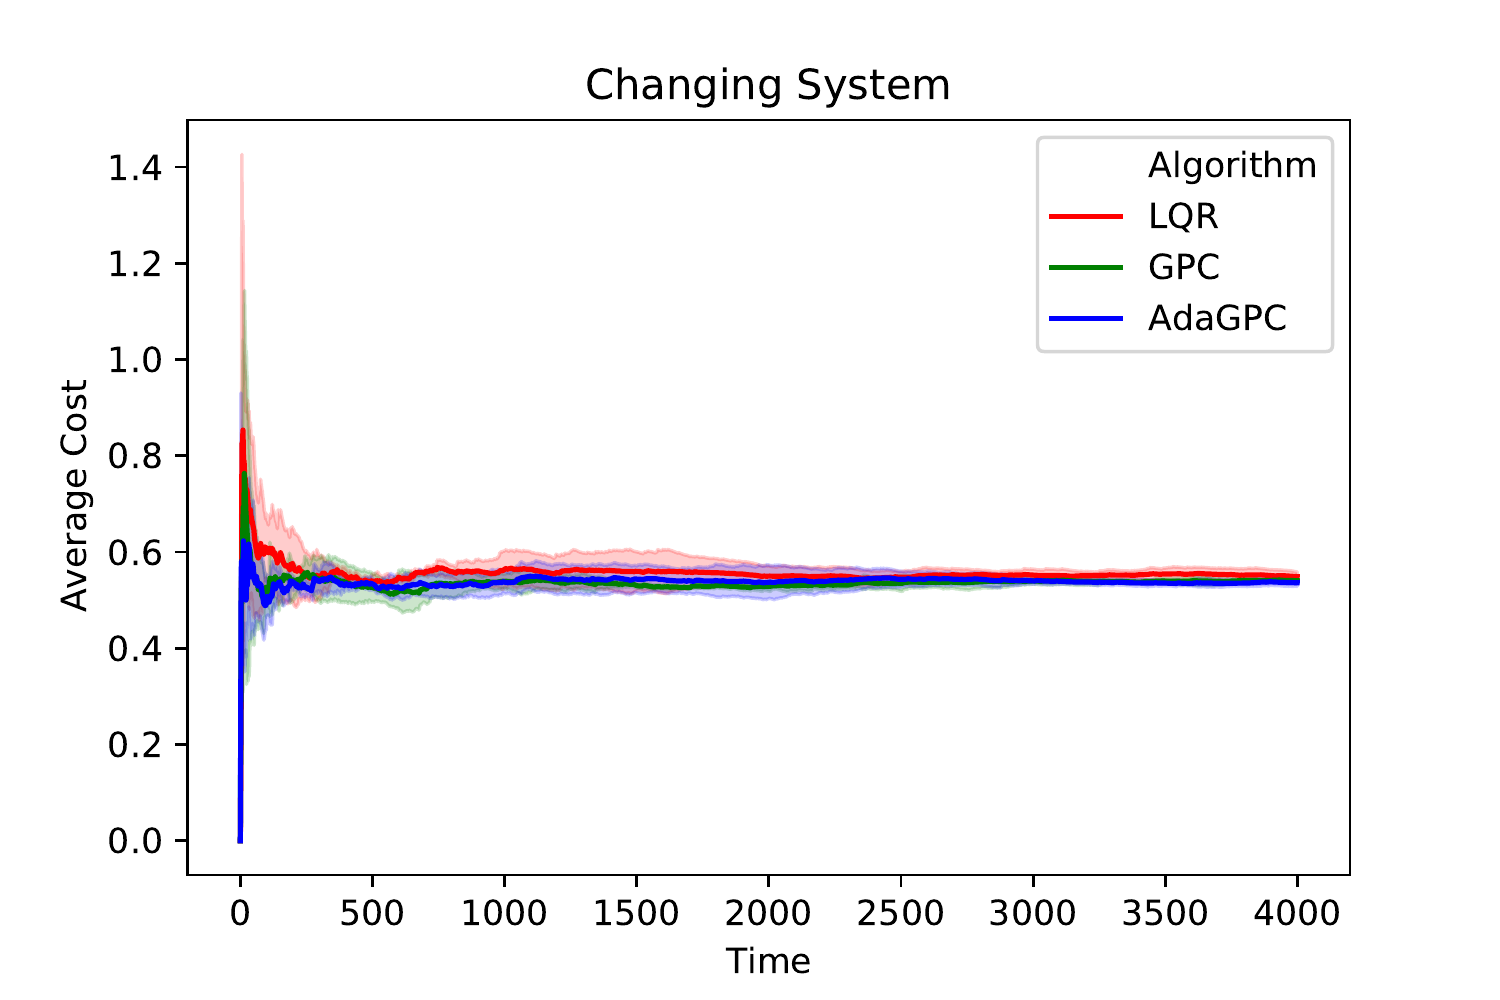}}
\caption{Performance comparison on systems (\ref{fixed_system}), (\ref{switching_system}), (\ref{changing_system}) under i.i.d Gaussian noise} \label{fig:experiments_gaussian}
\end{figure}

\paragraph{II. Alternating Noise.} For our second experiment (the one also illustrated in the main body of the paper), the same systems experience intermittent sinusoidal 'shocks'. Concretely, the perturbations alternate between (i) i.i.d. Gaussian [$w_t \sim \mathcal{N}(0, 0.3^2)$], and (ii) sinusoidal [$w_t[i] = sin((n*t + i)/(8\pi)$ where $w_t[i]$ is the $i^{th}$ entry of $w_t$ and $n$ is the state dimension]. This setting requires the controller to recognize changing conditions and quickly switch between "good-time" and "bad-time" policies at any point during learning. The task is even more compelling when we consider acting in systems with switching or changing dynamics (described below), as it requires also dealing with the potentially differing effect shocks have depending on the overarching system.

\begin{figure}[H]
\centering
\subfigure{\includegraphics[width=60mm]{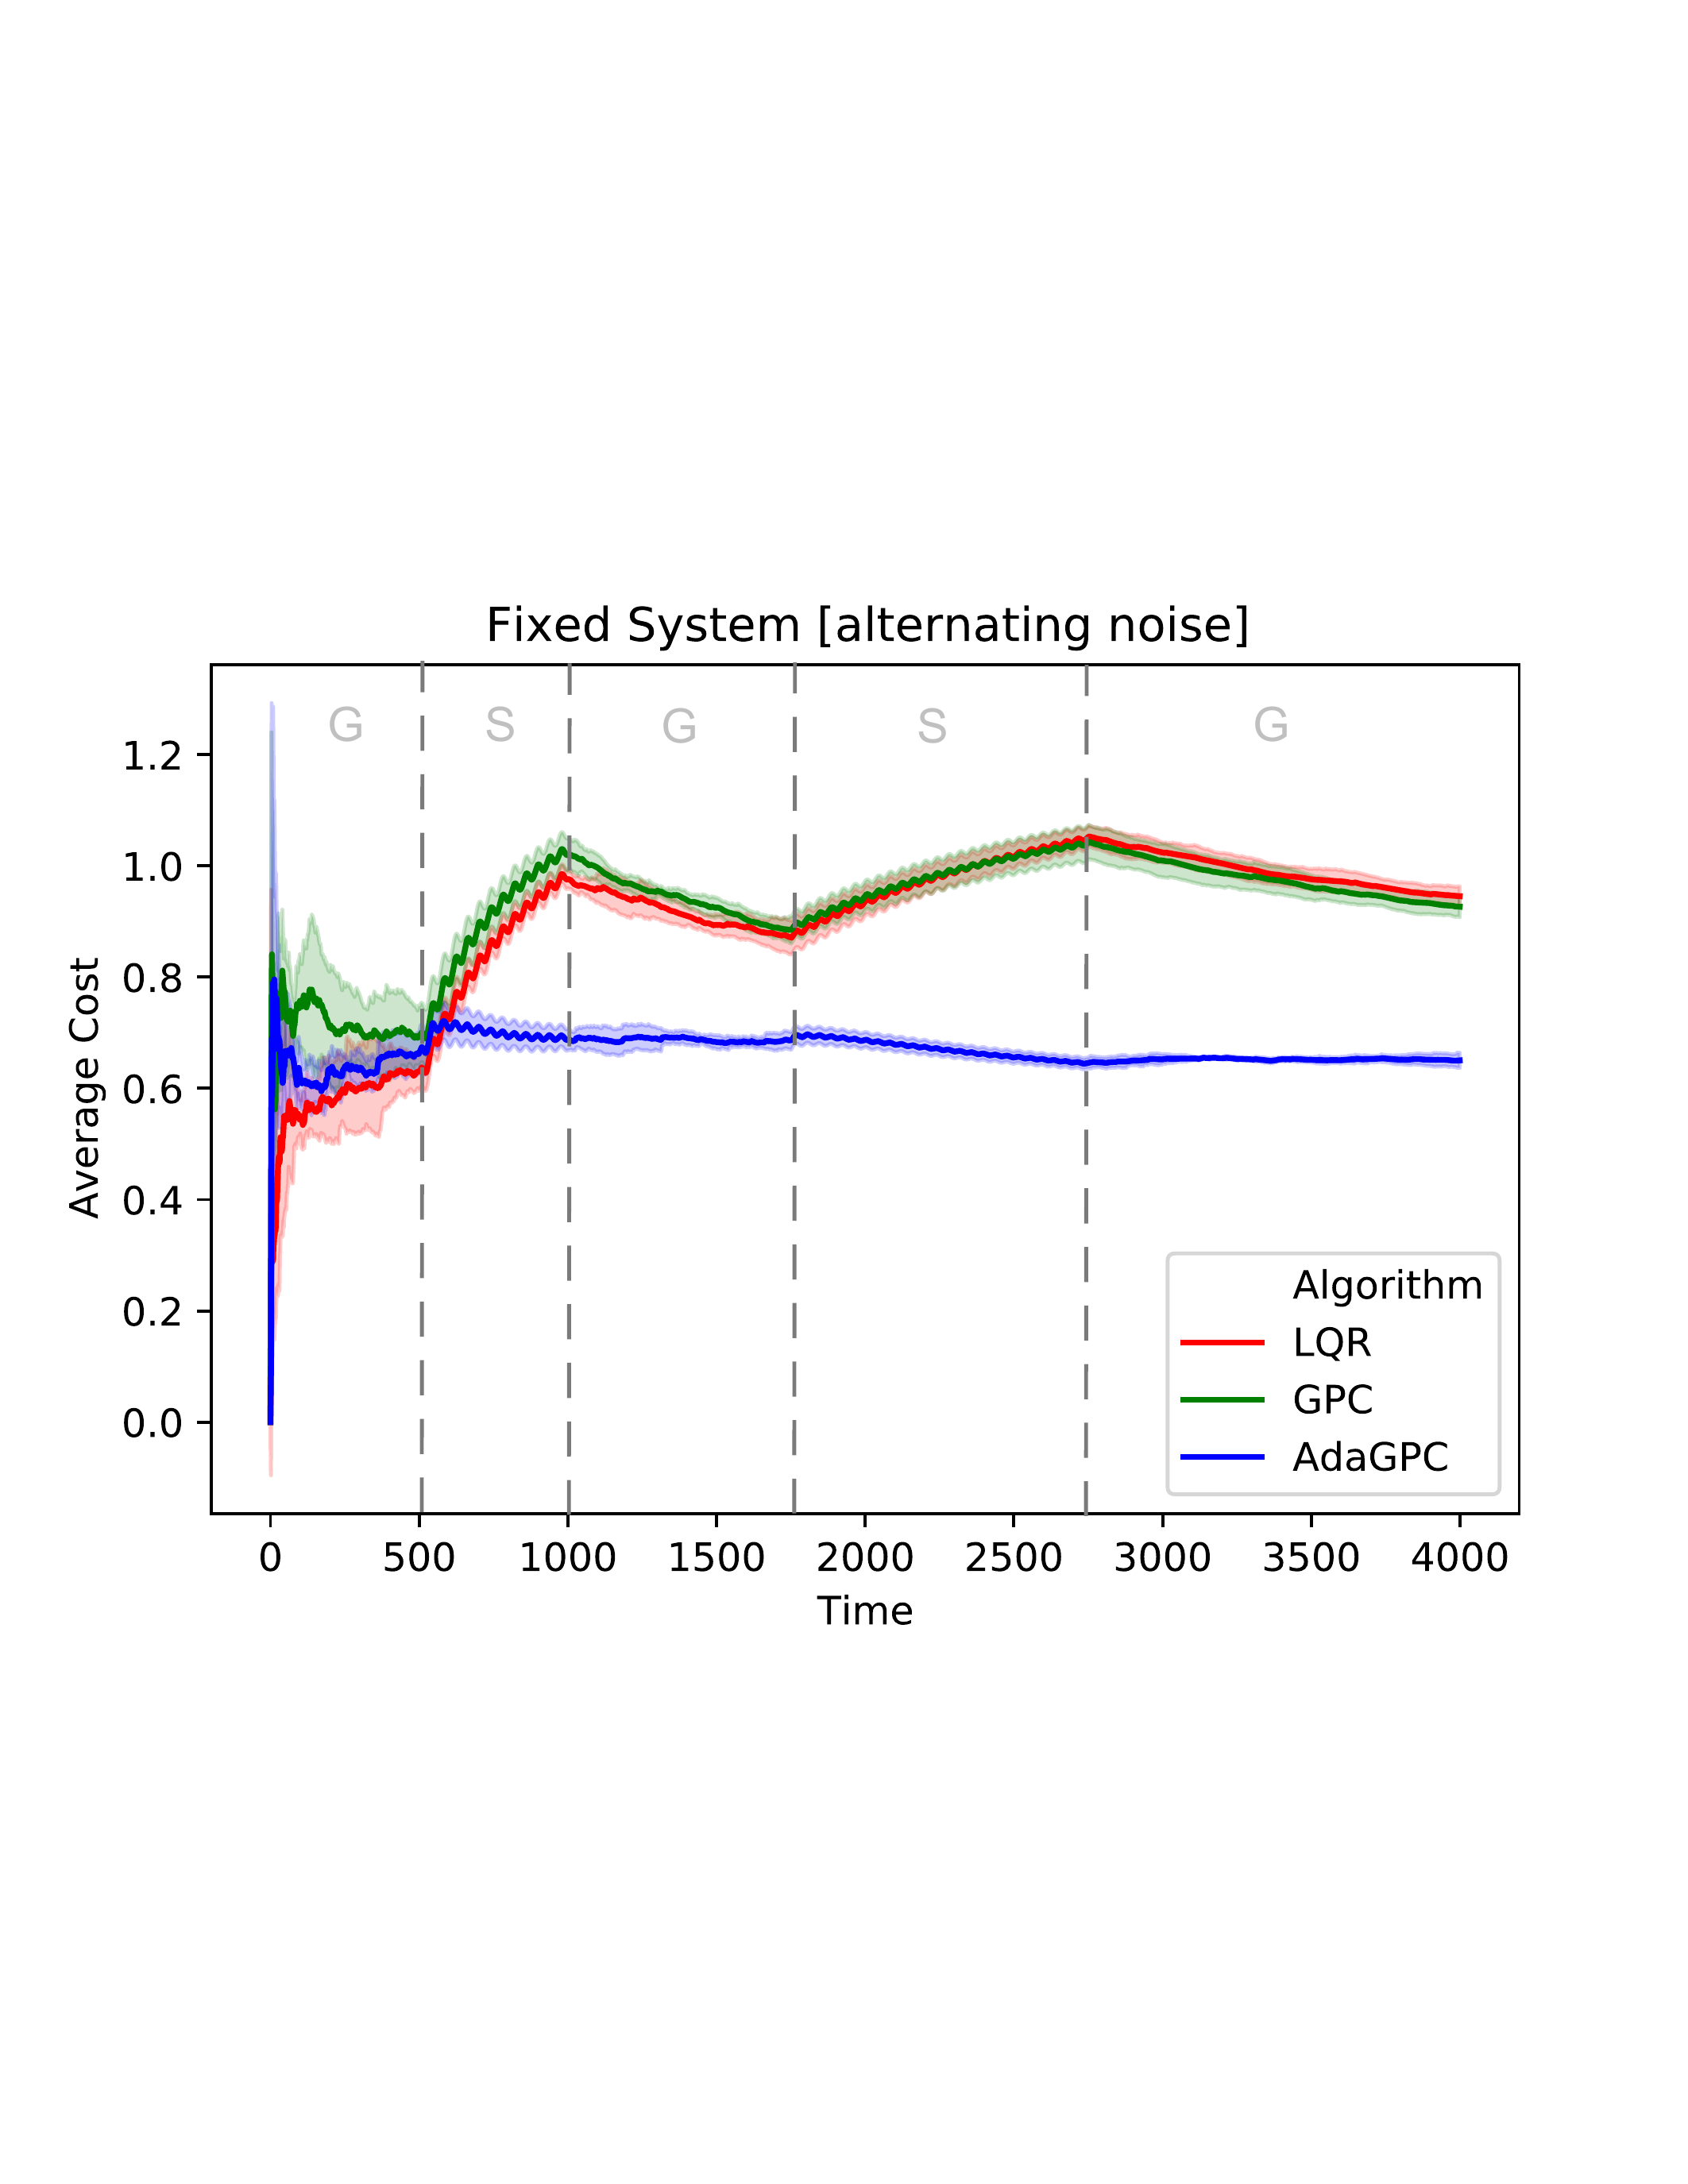}}
\subfigure{\includegraphics[width=60mm]{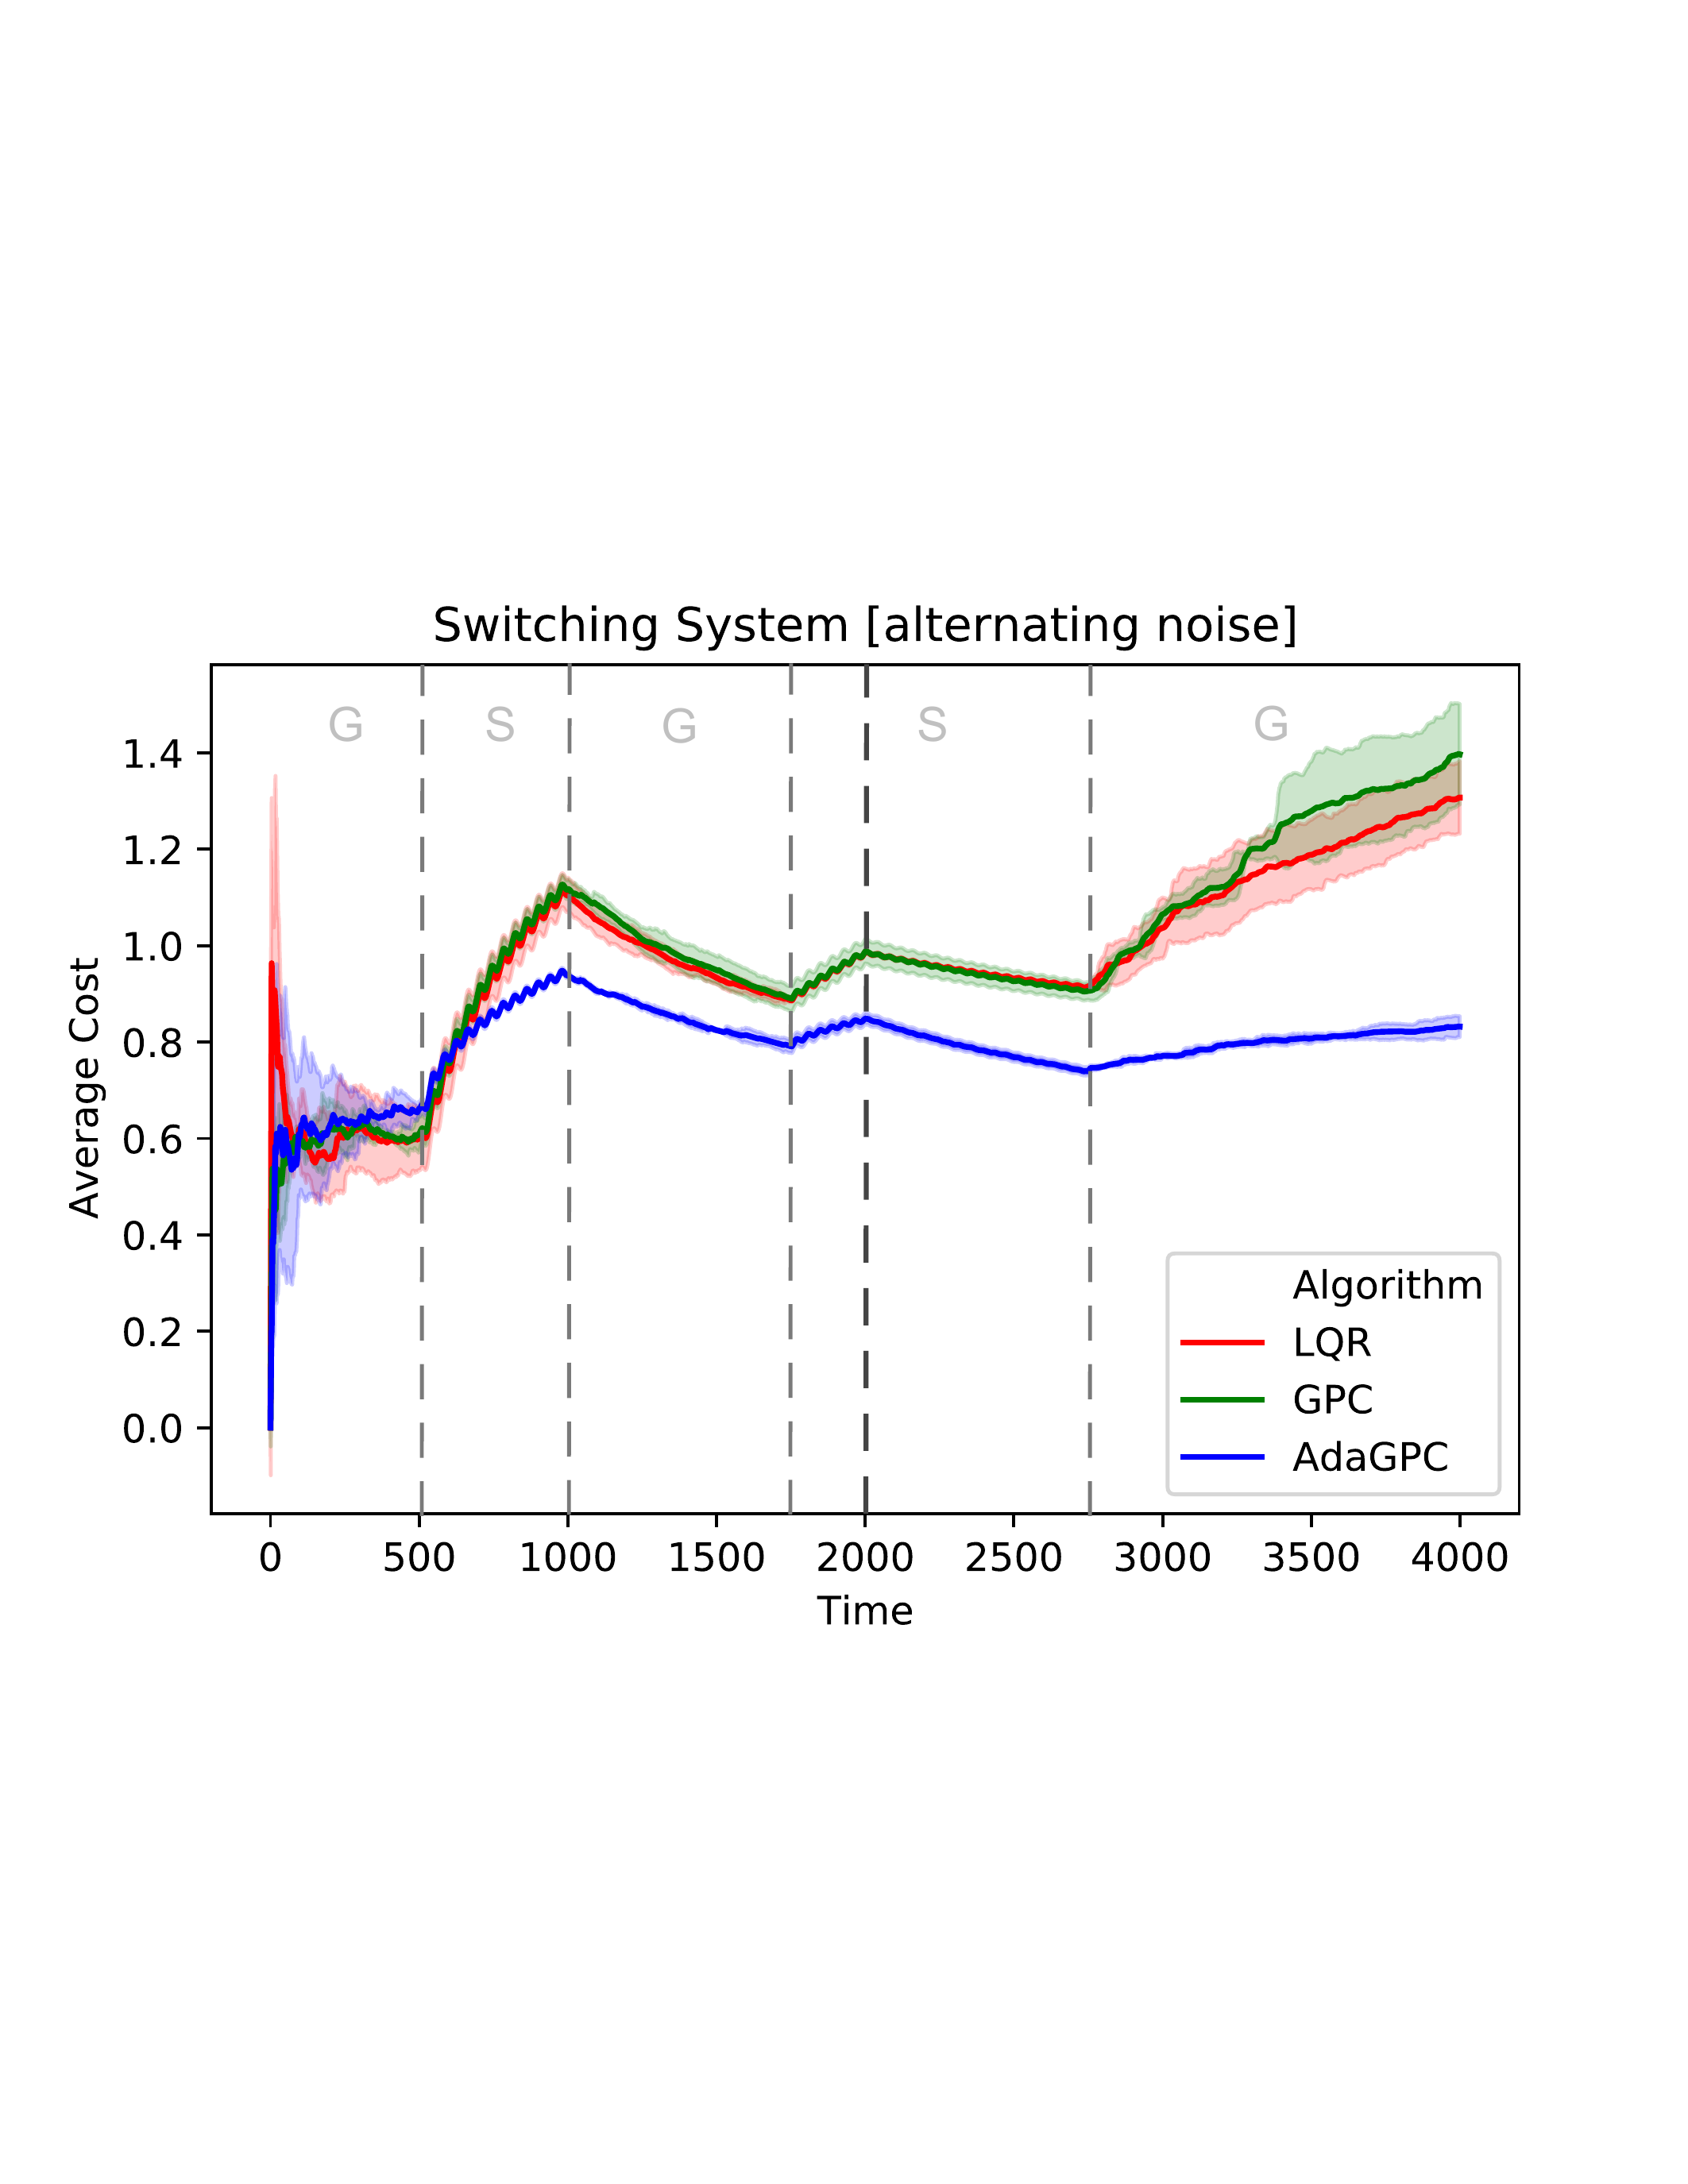}}
\subfigure{\includegraphics[width=60mm]{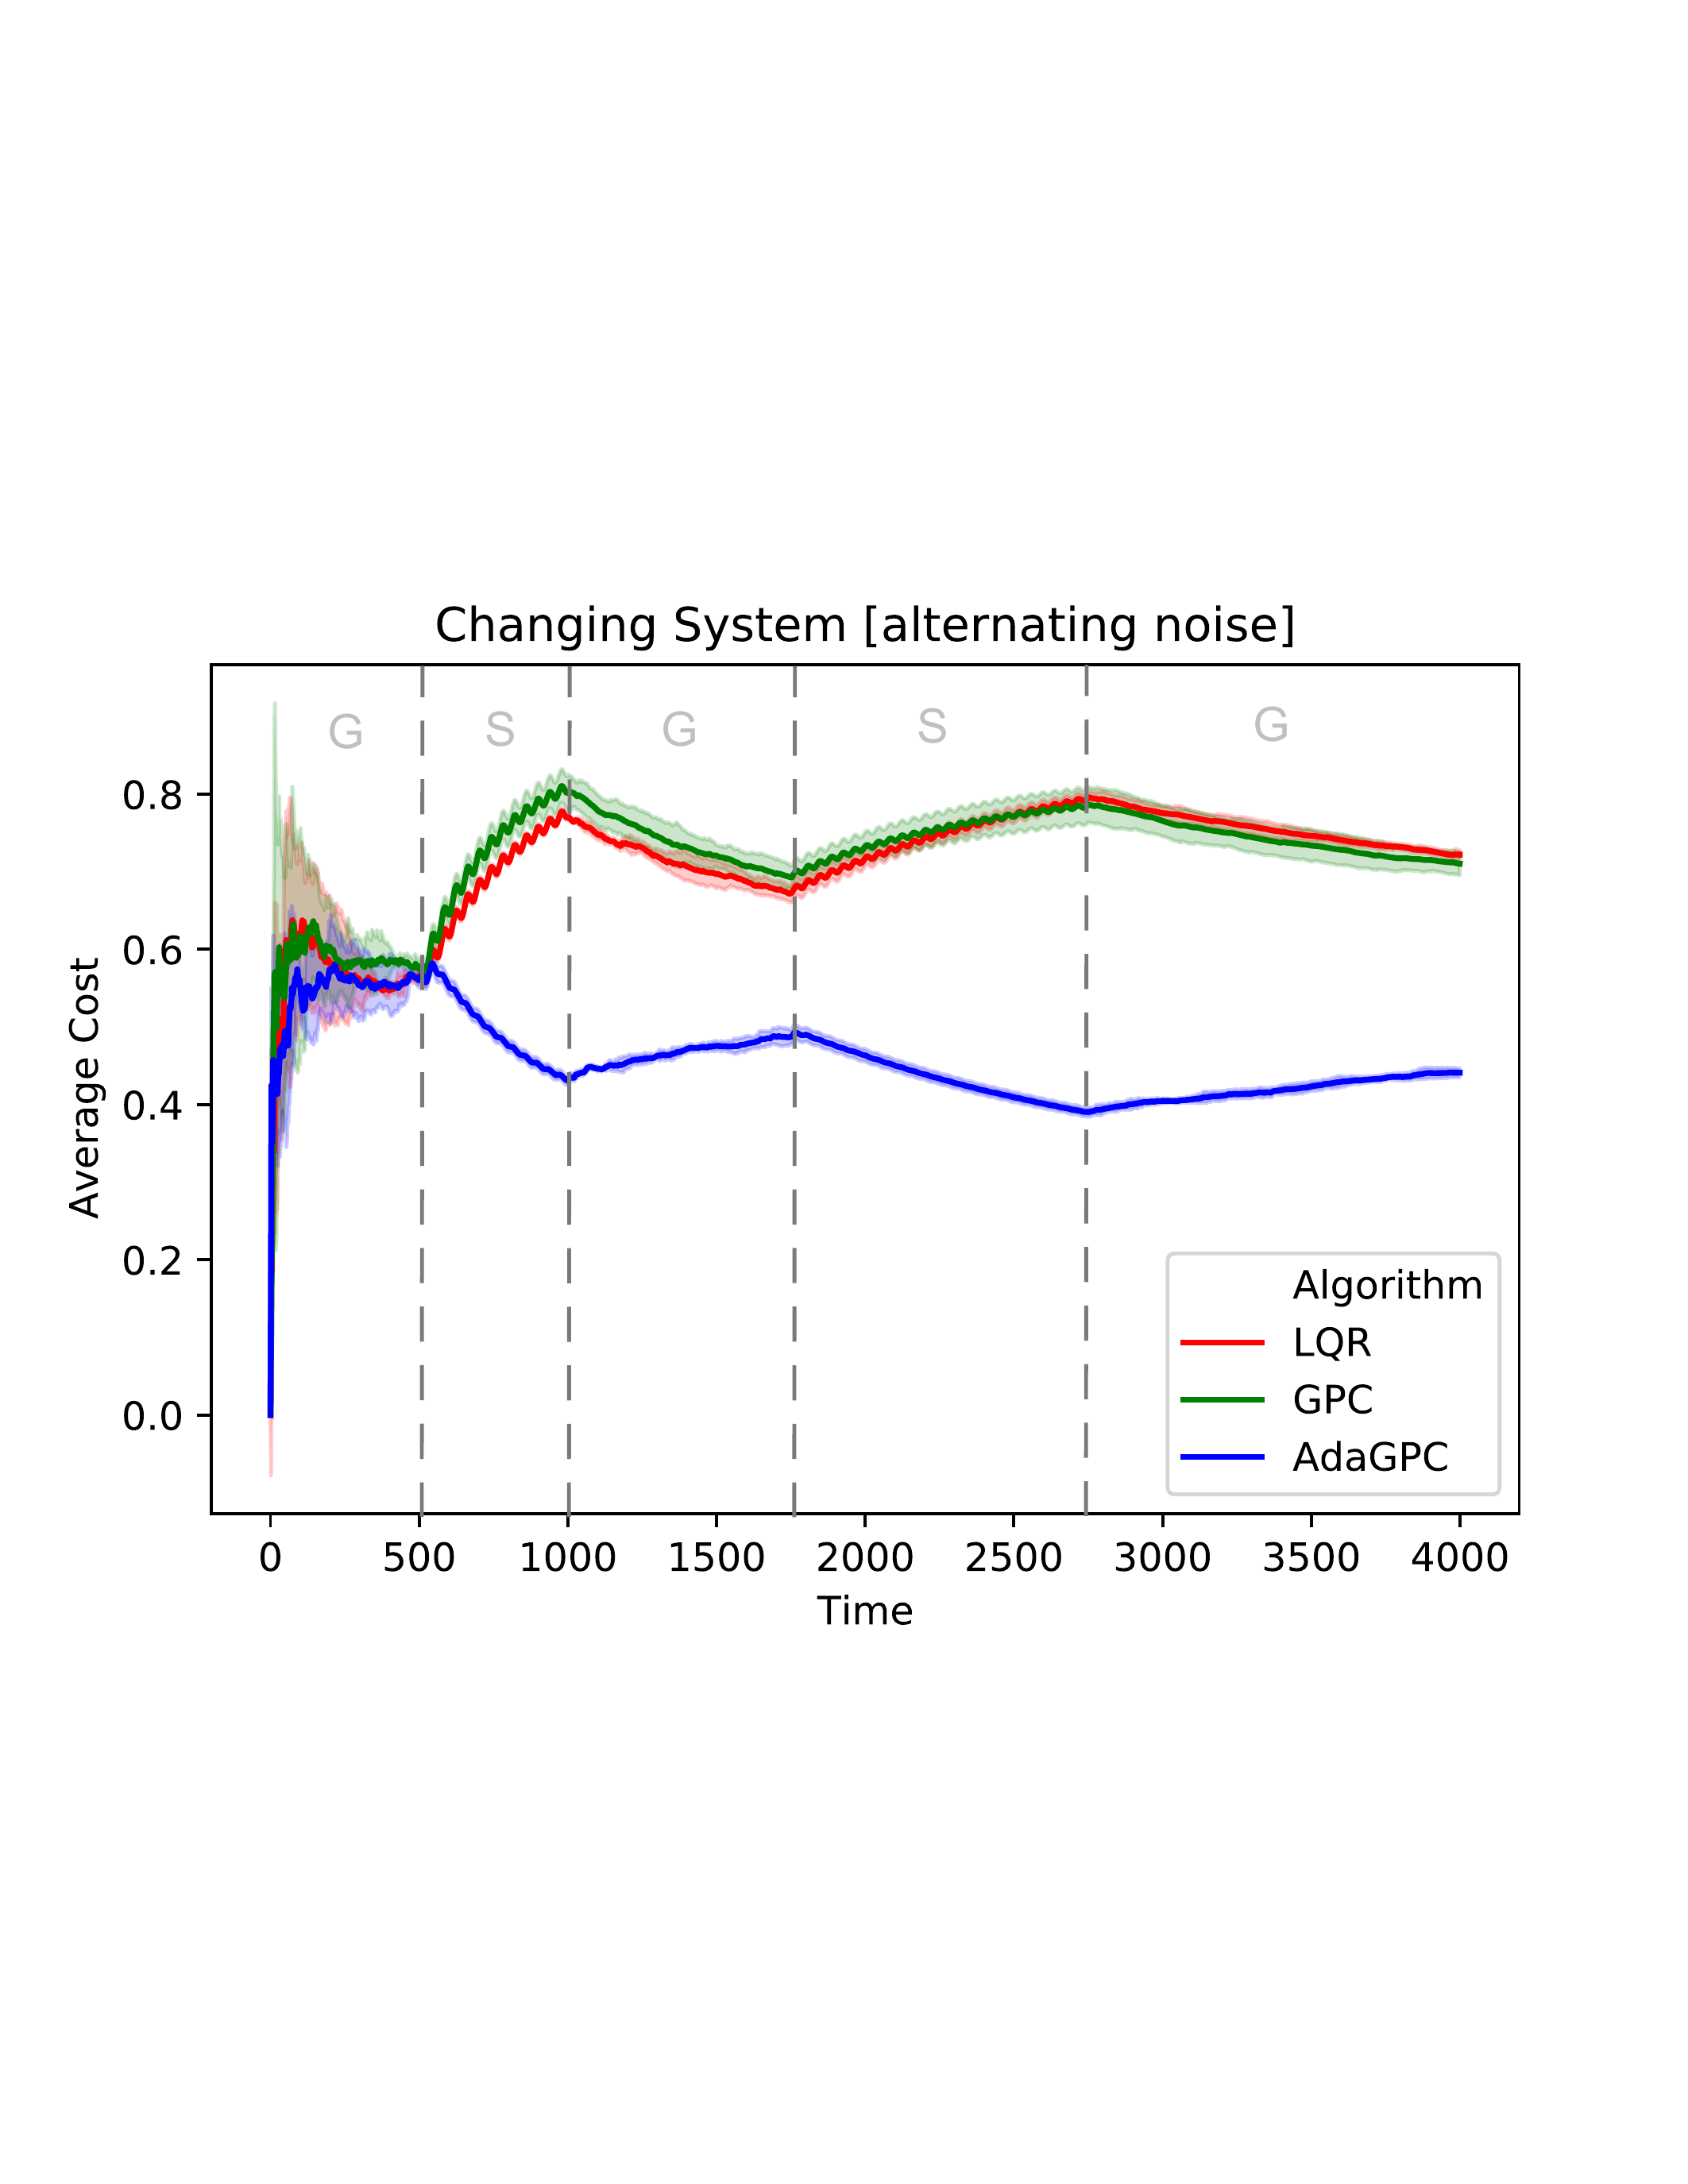}}
\caption{Performance comparison on systems (\ref{fixed_system}), (\ref{switching_system}), (\ref{changing_system}) under alternating noise distributions}\label{fig:experiments_5noise}
\end{figure}

As we can see in figures \ref{fig:experiments_gaussian} and \ref{fig:experiments_5noise}, our algorithm is able to quickly and effectively adapt to changing dynamics and perturbations, which validates our theoretical findings. Note that all $3$ algorithms perform similarly at first under Gaussian noise, but AdaGPC shows to be more robust to subsequent system and noise changes.

\subsection{Inverted Pendulum Experiment} \label{sec:exp_pendulum}

%\begin{figure}[H]
%\centering
%    \includegraphics[width=0.5\linewidth]{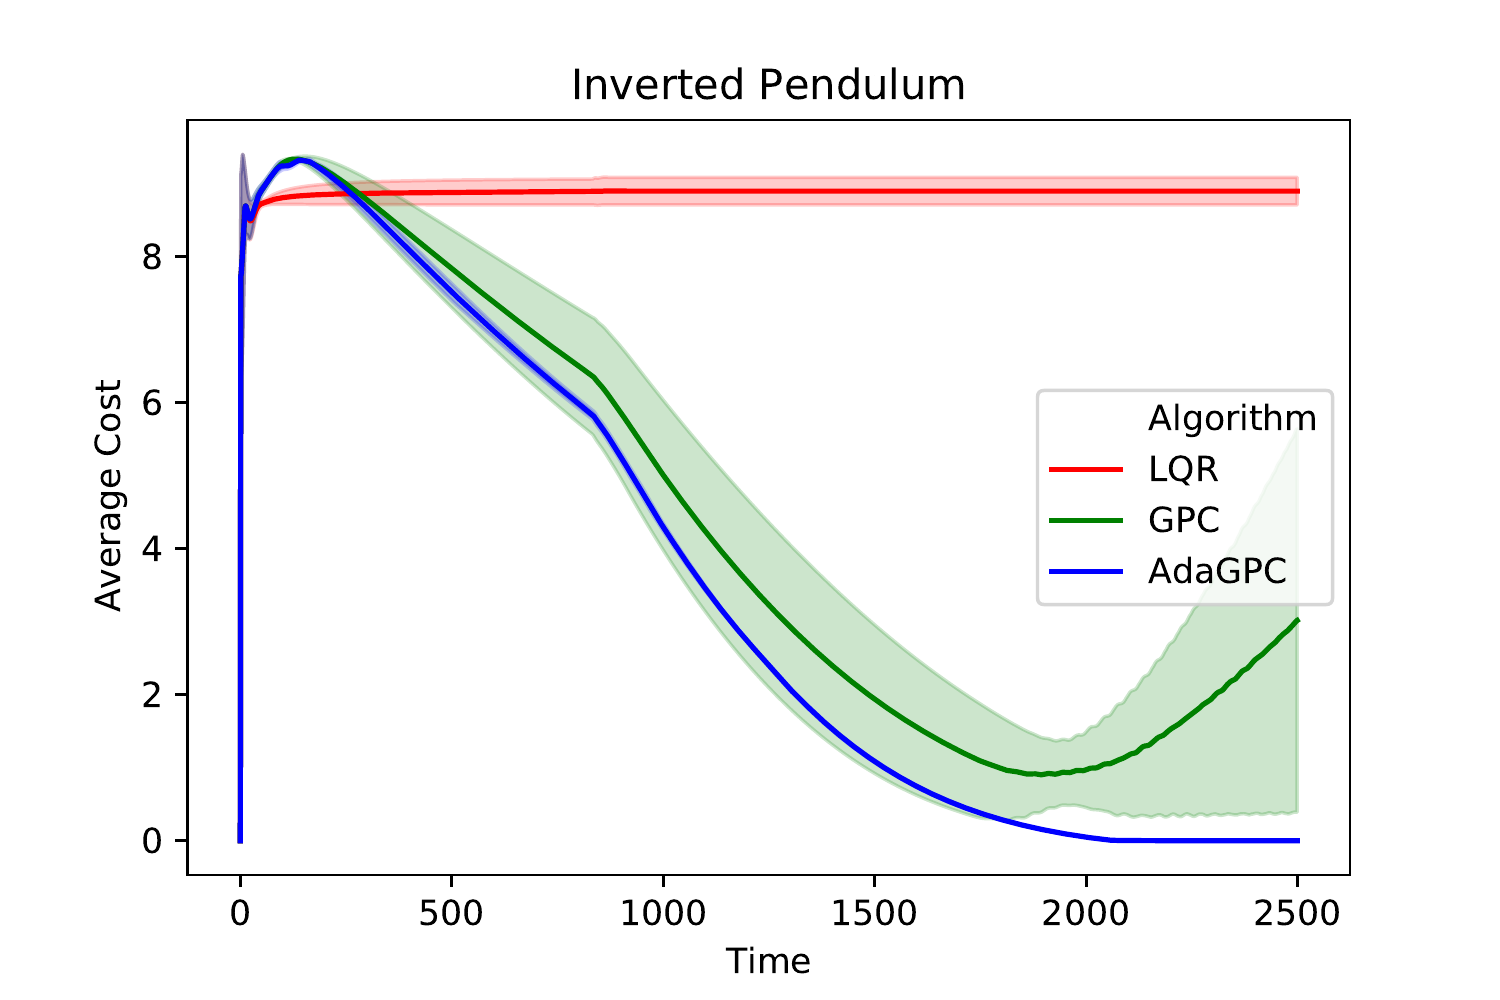}
%    \caption{Performance comparison on inverted pendulum}
%    \label{experiments_pendulum}
%\end{figure}

To show the applicability of our algorithm in more realistic (and harder) scenarios, we experiment on the inverted pendulum environment, a commonly used benchmark consisting of a nonlinear and unstable system, popularized by OpenAI Gym \citep{brockman2016openai}. 

\paragraph{Task.} For this system, the state consists of the deviation angle $\theta$ and the rotational velocity $\dot{\theta}$, while the action corresponds to the applied torque $\ddot{\theta}$. The objective is to balance the inverted pendulum by applying torque that will stabilize it in a vertically upright position. At each timestep, the learner incurs a cost of $\theta^2 + 0.1 \cdot \dot{\theta}^2 + 0.001 \cdot \ddot{\theta}^2$, where $\theta$ is normalized between $-\pi$ and $\pi$.

\paragraph{Technical Details.} We follow the dynamics and cost specification implemented in \cite{brockman2016openai} to model the task described above. In the figures below, we plot the instantaneous\footnote{We include instantaneous plots as they are particularly suited for visualizing the time required to solve the task.} and sliding window averaged\footnote{At time $t$, we plot the average cost incurred over the past $\min\{t, T//3\}$ iterations. We opt to include this specific metric, a trade-off between instantaneous and cumulatively averaged costs, as it can nicely capture both smoothed long-term behavior as well as convergence at the end of the run.} costs incurred by the controllers.

\paragraph{Competing against a strong baseline.} As a stronger comparator, we consider the classic planning algorithm iLQR and improve upon it using the techniques described in \cite{iLQR}, namely (1) optimizing over regularization terms and (2) introducing a backtracking line search parameter that protects against divergence. Figure \ref{pendulum} showcases the strength of the chosen baseline on our task (in the absence of noise).

\paragraph{I. Noiseless Dynamics} We first experiment with the original noiseless system. In figure \ref{pendulum} below, we see that our method enables a controller originally developed for linear systems (GPC) to be used to solve this harder, non-linear task. A less straight-forward benefit of our algorithm is that it enables the use of a larger learning rate in the base controller without the commonly associated unstable behavior (clearly displayed by GPC in the graph on the left). As the instantaneous cost graph illustrates, this allows AdaGPC to also converge fast to the solution, only slightly slower than our strong iLQR baseline.

\begin{figure}[H]
\centering
\subfigure{\includegraphics[width=60mm]{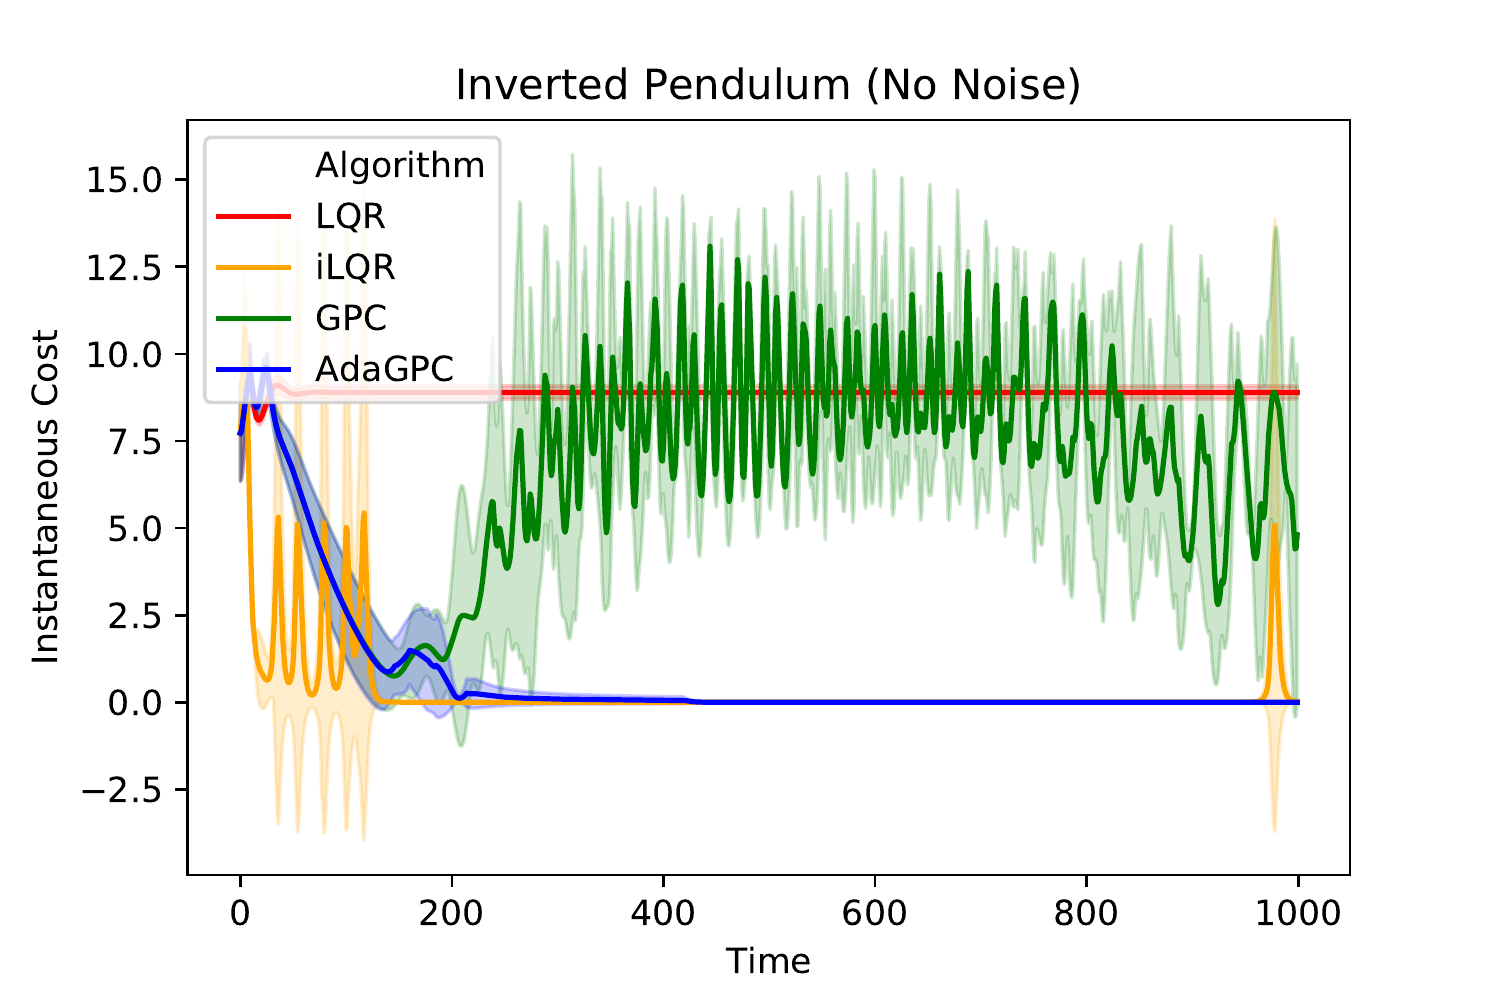}}
\subfigure{\includegraphics[width=60mm]{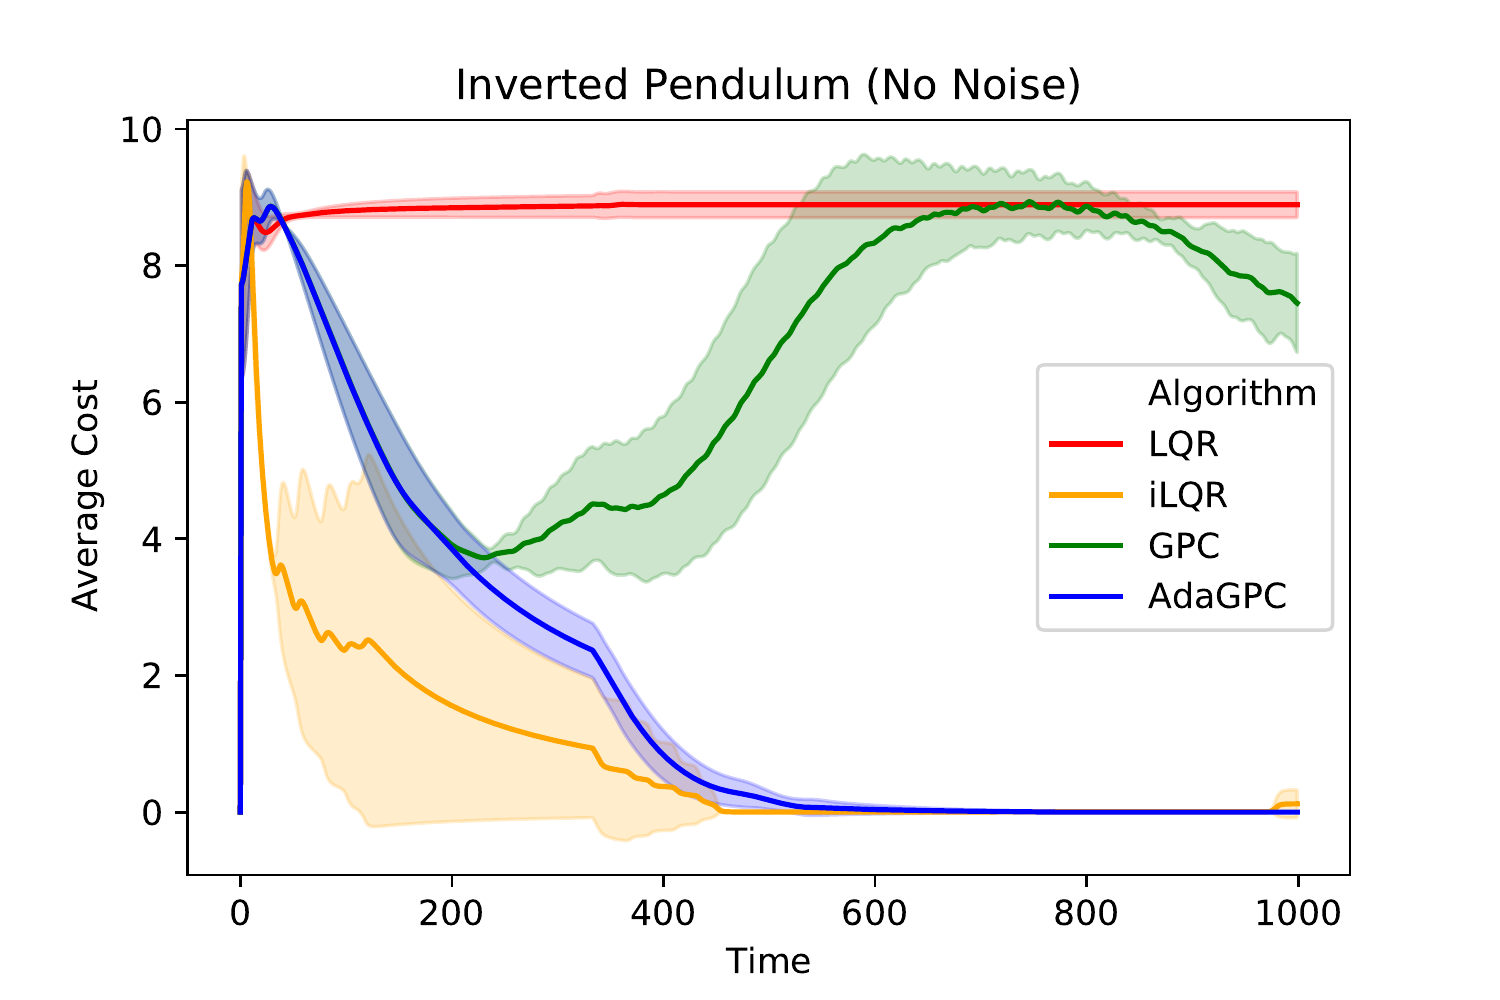}}
\caption{Performance comparison on a noiseless pendulum environment. Instantaneous cost is plotted in the left graph and the sliding window averaged cost is plotted in the right graph.} \label{pendulum}
\end{figure}

\paragraph{II. Sinusoidal Shock} We further complicate the original task by introducing a sinusoidal shock in the middle of the run. We ideally desire a controller that is able to recover from such an adverse shock and re-stabilize the pendulum. In figure \ref{pendulum_sine}, we see that our strong iLQR planner is unable to adapt to an unanticipated shock due to its static and environment-agnostic design. However, thanks to its ability to respond to what is actively happening in the environment, our method succeeds at this new harder task. 

\begin{figure}[H]
\centering
\subfigure{\includegraphics[width=60mm]{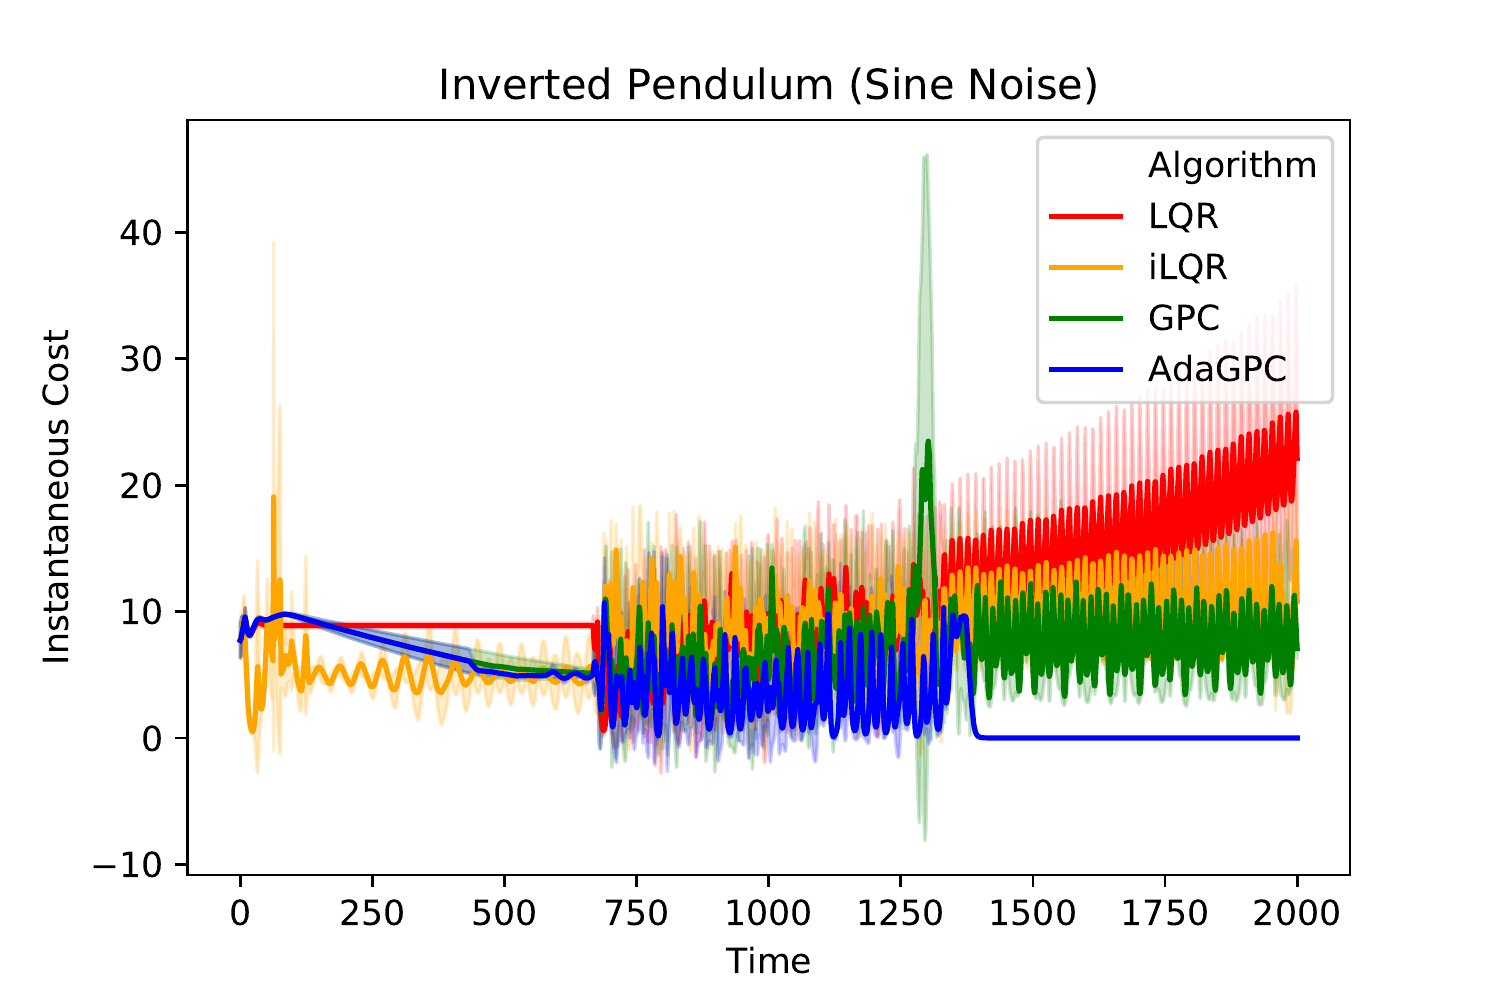}}
\subfigure{\includegraphics[width=60mm]{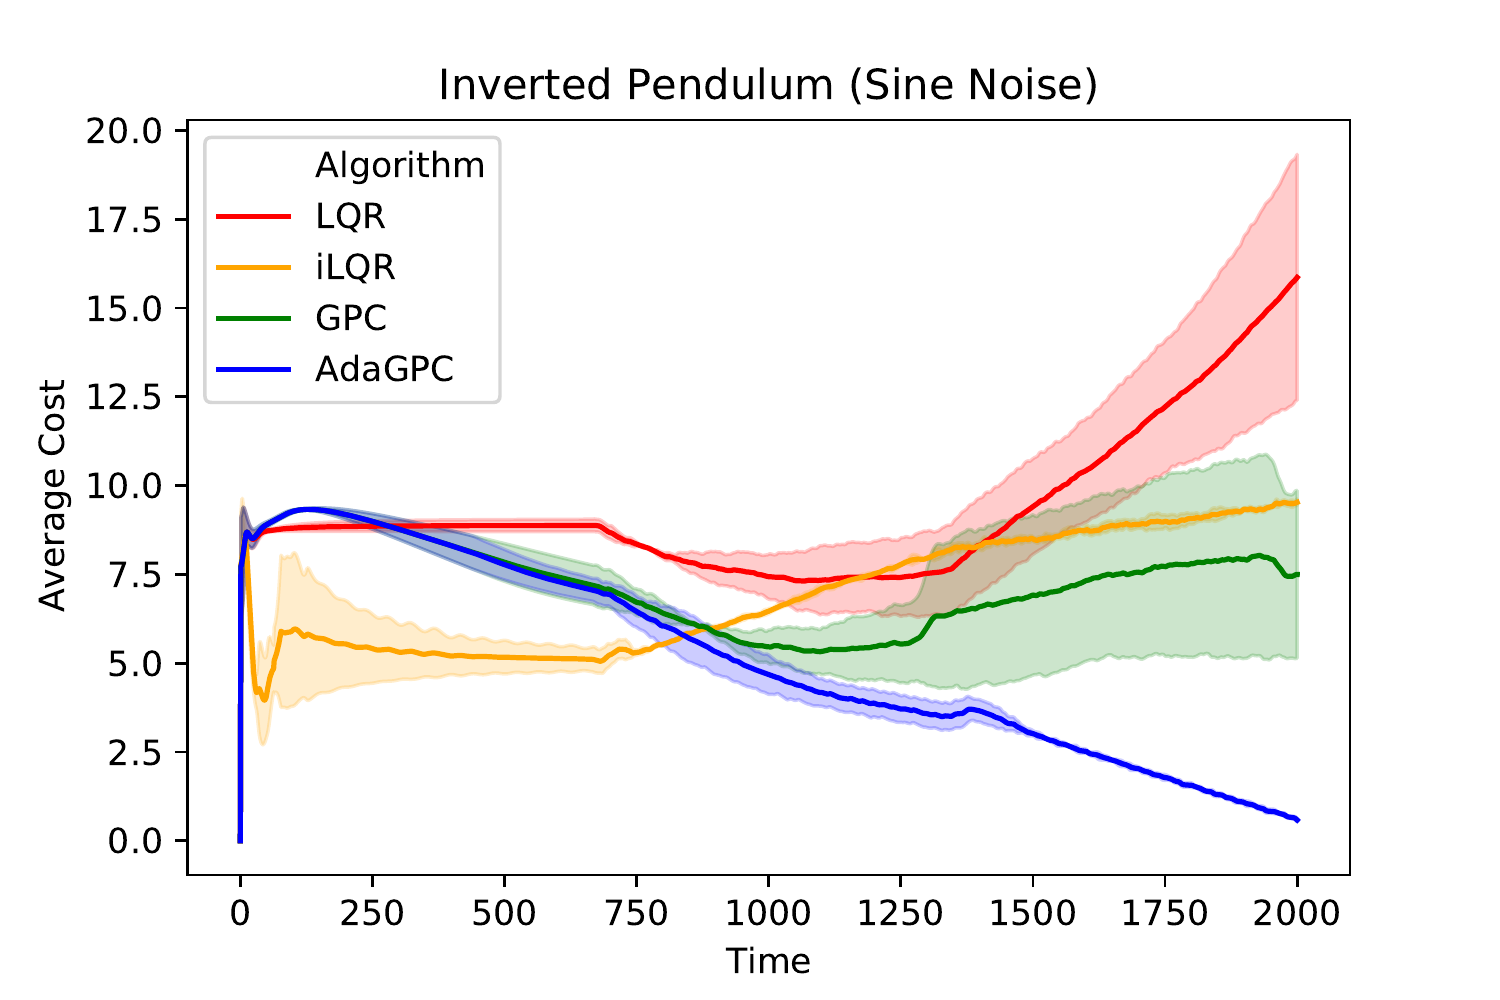}}
\caption{Performance comparison on a pendulum environment experiencing a midway sinusoidal shock. Instantaneous cost is plotted in the left graph and the sliding window averaged cost is plotted in the right graph.}\label{pendulum_sine}
\end{figure}

These results confirm that the proposed approach is highly promising even from a practical standpoint, and provides a viable alternative to the classic planning approach.
