# Supplementary material for: Adaptive Regret for Control of Time-Varying Dynamics
Source: arXiv:2007.04393 source file (2022-02-12)
Supplement: Supplementary file 2 [file smooth-systems.tex]

\section{Smooth dynamical systems}

Let $f : \R^{d_x} \times \R^{d_u} \mapsto \R^{d_x} $ be a dynamical system. 
Let $\pi:  \R^{d_x} \mapsto \R^{d_u} $ be a policy in the same space, and let $g: \R^{d_x} \mapsto \R^{d_x}$ denote the dynamics arising by applying $\pi$ to $f$. The dynamics are given by the following equation,
\begin{equation*}
    x_{t+1} = f(x_t, u_t) + w_t ~.
\end{equation*}
The iterative linearization technique gives rise to the state and action matrices that are time-varying: $A_t = \nabla_{x_t} f \in \R^{d_x \times d_x}$ and $B_t = \nabla_{u_t} f \in \R^{d_x \times d_u}$. We clarify this notation given that $f$ is a vector-valued function: for a vector-valued $f : \R^d \to \R^p$ and a vector point $v \in \R^d$, denote $G = \nabla_v f \in \R^{p \times d}$ where the $i$'th row is $G[i, :] = \nabla_v f_i$ for $i \in [p]$. \eh{the standard name for this is the Jacobian} \edgar{hahah, yes of course...}

The aforementioned notation allows us to express the non-linear dynamics in terms of time-varying linear dynamics and an additional second order error which we assume to be small:
\begin{equation*}
    x_{t+1} = A_t x_t + B_t u_t + v(x_t, u_t) + w_t,
\end{equation*}
where $v(x, u)$ is the second order approximation error of the dynamics function $f$, i.e. $v(x, u) = f(x, u) - \left[\nabla_{x, u} f\right]^{\top} [x, u]$. We assume this error is small at all times during the control sequence, more generally $\| v(x, u) \| \leq \eps$ for all $x \in \R^{d_x}, u \in \R^{d_u}$. This does not mean $f$ is close to being a linear function as in such a case the gradient itself would not change over time.

Ideally, we would want the rate of change $\xi$ of $(A_t, B_t)$ as defined above to be small, e.g. $\xi = O(T^{-1})$. Note that if $f$ is smooth (similar to what is defined below), then $A_{t+1} - A_t = \nabla_{x_{t+1}} f - \nabla_{x_t} f$ is small in magnitude if $\|x_{t+1}-x_t\|$ is small. Same applies for $B_t$ and $u_t$. The iterative movement in state and/or action being sublinear in $T$ for all $t \in [T]$ does not seem to be a feasible thing to prove. \eh{Not sure I agree:  IMO the change $\|x_t - x_{t-1}\| \sim \eta$, where $\eta$ is the learning rate, and usually sublinear} \edgar{this is not OGD so i don't think that's true, we should discuss}

However, there seems to be an easy workaround for this issue. Recall that having a small rate of change is {\it not} necessary. If we show that $\|A_t - A_r\|$ is small (small means $O(1)$ in this case) for all $t \in I = [r, s]$ given any arbitrary subinterval $I = [r, s]$, then the argument from \ref{sec:slow_known} still holds. A smoothness assumption for $f$ gives us $\| A_t - A_r \| \leq \beta \| x_t - x_r \|$. Given that the magnitude bound holds for both states and actions this trivially gives us $\| x_t - x_r \| \leq 2 D_x$ and we can conclude that $\| A_t - A_r \| = O(1)$ for all $t \in I$, any fixed $I = [r, s] \subseteq [T]$. The exact same argument holds for the action space, and gives $\| B_t - B_r \| = O(1)$. \eh{IMO E3 and this section needs to be merged. The treatment here is the more general one.} \edgar{sure, that's not an issue; we presented E.3 that way so the slowly changing name makes sense}

TODO: check that the magnitude bound still holds in this case (or what assumptions are necessary).

Let $g_i : X \mapsto \reals$ be the projection of $g$ onto the $i$'th coordinate. 

We say that $g$ is $\beta$-smooth over $K \subseteq \reals^d$ iff 
$$ \forall i \in [d], x \in \K \ . \  \| \nabla^2 g_i\| \leq \beta $$

TODO:
\begin{enumerate}
    \item Show that this definition implies that the gradients of $g$ are $\beta$-Lipschitz. 
    \item Therefore, iterative linearization means that $A_t,B_t$ change slowly.
\end{enumerate}
