# Supplementary material for: Adaptive Regret for Control of Time-Varying Dynamics
Source: arXiv:2007.04393 source file (2022-02-12)
Supplement: Supplementary file 3 [file setting.tex]

\section{Formal Assumptions}\label{sec:assmpts}

\paragraph{Online convex optimization with memory.}
We address the problem of online control of a linear dynamical system from the setting of online convex optimization (OCO, see e.g. \cite{hazan2016introduction}), and specifically OCO with memory.  In this setting, at each round $t = 1, 2, \dots$ the online player chooses an action $\x_t \in \mathcal{K}$ from the decision set $\mathcal{K} \subset \R^d$ and after committing to that action observes the loss function $f_t : \mathcal{K} \to \R$ suffering loss $f_t(\x_t)$. In many environments the decisions of the player affect the long-term future, such is the case in the problems of control and reinforcement learning. Hence, in the setting with memory the adversary reveals the loss function $f_t : \K^{H+1} \mapsto \reals$ that applies to the last $H+1$ decisions of the player, and the player suffers loss $f_t(\x_{t-H:t})$ where $\x_{i:j} = \{\x_i, \dots, \x_j\}$ with $i < j$. Define the surrogate loss $\tilde{f}_t : \mathcal{K} \mapsto \R$ to be the function with all $H+1$ arguments equal, i.e. $\tilde{f}_t(\x) = f_t(\x, \dots, \x)$. The regret in this setting is defined with respect to the best surrogate loss in hindsight as follows, where we denote $\x_i = \x_1$ for all $i < 1$,
\begin{equation*}
    \regret = \sum_{t=1}^T f_t(\x_{t-H:t}) - \min_{\x \in \mathcal{K}} \sum_{t=1}^T \tilde{f}_t(\x) ~.
\end{equation*}

We henceforth denote the diameter of the set $\K$ by $D$, and the bound on the Euclidean norm of the gradients of the surrogate loss functions by $G$. Notice that the given definition reduces to the standard regret setting when $H=0$.

% \subsection{Adaptive regret} 
\paragraph{Adaptive regret.}
It has been observed in the literature that the standard regret benchmark promotes convergence to the static optimum of the entire learning sequence, and in certain cases hinders adaptivity to changing environments. To remedy this situation, \cite{hazan2009efficient} suggest a more refined metric, called adaptive regret, which promotes adapting to environment changes. The metric captures the supremum over all local regrets in any contiguous time interval: formally, for an online algorithm $\A$ over $T$ rounds with actions $\{\x_t\}_{t \in [T]}$ in response to losses $f_1, \dots, f_T$, denote
\begin{equation*}
\adreg_{\mathcal{A}}(T) = \sup_{f_1, \dots, f_T} \sup_{[r, s] = I \subseteq [T]} \left[ \sum_{t=r}^s f_t(\x_t) - \min_{\x^\star_I \in \mathcal{K}} \sum_{t=r}^s f_t(\x^\star_I) \right] ~.
\end{equation*}

The strength of this definition is that it does {\it not} try to model the environment. Instead, it shifts responsibility to the learner to try to cope with the best local predictor $\x^\star_I$ for every time interval $I$. This metric was shown to be meaningful for both abrupt changes as well as slowly changing environments. We analogously denote $\reg_{\A}(T)$ to be the supremum of standard regret over $f_1, \dots, f_T$ adversarially chosen losses. Finally, define the notion of {\it action shift} as the overall shifting in distance of consecutive actions by $\A$, i.e. %For example, an abrupt change in environment can be captured by a local optimum change. But much more generally, the environment can change arbitrarily slow or fast, and as long as the best time-local optimum performs well, an adaptive regret algorithm can perform as well as this locally-optimal decision. 
\begin{equation*}
     \shift_{\A}(T)  = \sup_{f_1, \dots, f_T} \sum_{t=1}^{T-1} \| \x_{t+1} - \x_t \| ~.
\end{equation*}

The following well-known facts are stated below for further reference (see appendix for proofs).
\begin{fact}\label{claim:scogd}
Let $\A_{\text{scOGD}}$ be the projected OGD algorithm over $\alpha$-strongly convex loss functions with stepsizes $\eta_t = \frac{1}{\alpha t}$, then $\reg_{\A_{\text{scOGD}}}(T)  = O(\frac{G^2}{\alpha} \log T)$ and $\shift_{\A_{\text{scOGD}}}(T)  = O(\frac{G}{\alpha} \log T)$.
\end{fact}
\begin{fact}\label{claim:cogd}
Let $\A_{\text{cOGD}}$ be the projected OGD algorithm over general convex loss functions with stepsizes $\eta_t = \frac{D}{G \sqrt{t}}$, then $\adreg_{\A_{\text{cOGD}}}(T)  = O(D G \sqrt{T})$ and $\shift_{\A_{\text{cOGD}}}(T)  = O(D \sqrt{T})$.
\end{fact}

\subsection{Control of linear dynamical systems}\label{sec:setting_control}

In this paper we consider adaptive online control, and therefore changing dynamical systems. A time-varying linear dynamical system is given by the following dynamics equation,
\begin{equation*}
x_{t+1} = A_t x_t + B_t u_t + w_t ,
\end{equation*}
where $x_t \in \R^{d_x}$ is the (observable) system state, $u_t \in \R^{d_u}$ is the control, and 
$(A_t, B_t)$ are the system matrices with $A_t \in \R^{d_x \times d_x}$, $B_t \in \R^{d_x \times d_u}$. The vector  $w_t \in \R^{d_x}$ is a bounded disturbance. 
In our work, we allow $w_t$ to be completely arbitrary. This additional generality allows the disturbance to model deviations from linearity, in addition to the changing linear dynamics. 

\ignore{
\eh{TEMP: 
It is shown in \citep{hazan2019nonstochastic} that for an unknown system $(A, B)$ and a known $(\kappa, \gamma)$ strongly stable controller $K$, a disturbance-action controller can achieve sublinear regret against all such controllers parametrized by $(K', M)$ where $K'$ is $(\kappa, \gamma)$ strongly stable.
\begin{definition}
A disturbance-action controller with parameters $(K, M)$ where $M = [M^0, M^1, \ldots, M^{H-1}]$ outputs control $u_t$ at state $x_t$,
$$ u_t = Kx_t + \sum_{i=1}^H M_{i-1} w_{t-i}. $$
\end{definition}}
}

We consider the setting of {\it known} systems, i.e. after taking an action $u_t$ the controller observes the next state $x_{t+1}$ as well as the current system matrices $(A_t, B_t)$. This allows the controller to compute the disturbance $w_t = x_{t+1} - A_t x_t - B_t u_t$, so the knowledge of $x_{t+1}$ and $w_t$ is interchangeable. 

A control algorithm $\mathcal{C}$ chooses an action $u_t = \mathcal{C}(x_1, \dots, x_t)$ based on previous information. It then suffers a cost of $c_t(x_t,u_t)$ according to a cost function $c_t$. The cost function can change arbitrarily with time, and we only assume it has domain $[0, 1]$. 
The performance metric of $\mathcal{C}$ over horizon $T$ is adaptive policy regret with respect to a class of policies $\Pi$ as defined in \eqref{eq:aregret}.

The target class of policies we compare against in this paper are disturbance action controllers (DAC), % strongly stable\footnote{strong stability is rigorously defined in the appendix and not required for the derivation of our main results.} 
whose control is a linear function of past disturbances plus a stabilizing linear operator over the current state $u_t = K x_t + \sum_{i=1}^H M_i w_{t-i}$, for some history-length parameter $H$. This comparator class is known to be more general than the state-of-the-art in linear control: linear dynamical controllers (LDC). This choice is a consequence of recent advances in convex relaxation for control  \citep{agarwal2019online,agarwal2019logarithmic,hazan2019nonstochastic,simchowitz2020improper}.  

To characterize the actions picked by a controller $\C$, one can simply take a subset of $\R^{d_u}$ as a constraint set. However, since the system changes over time, actions at different rounds might need different constraints. For this reason, we describe a more general treatment: fix an arbitrary horizon $T$, let $\mathcal{U}_t \subset \R^{d_u}$ be the constraint set for action $u_t$ by controller $\C$ for each $t \in [T]$. Denote the action set sequence $\mathcal{U}_{1:T} = \{\mathcal{U}_1, \dots, \mathcal{U}_T \}$ and use $u_{1:T} \in \mathcal{U}_{1:T}$ to indicate $u_t \in \mathcal{U}_t$ for all $t \in [T]$ where $\mathcal{U}_t$ potentially depends on the system up to time $t$.

\begin{definition}\label{def:membounded}
Given a control sequence $u_{1:T} \in \mathcal{U}_{1:T}$ and memory parameter $H$, for all $t>H$ define $\hat{x}_t$ to be the state reached by the system if we artificially set $x_{t-H} = 0$. The action set sequence $\mathcal{U}_{1:T}$ is said to have $(H, \eps)$-bounded memory if for all $u_{1:T} \in \mathcal{U}_{1:T}$ and $t \in [T]$, $t > H$
\begin{equation*}
    | c_t(x_t, u_t) - c_t(\hat{x}_t, u_t) | \leq \eps ~.
\end{equation*}
\end{definition}

Suppose an action set sequence $\mathcal{U}_{1:T}$ has $(H, \eps)$-bounded memory. Then, given that $\hat{x}_t = \hat{x}_t(u_{t-H}, \dots, u_{t-1})$, the performance guarantees of a proxy cost function $f_t(u_{t-H:t}) = c_t(\hat{x}_t, u_t)$ imply guarantees for the control setting. In addition, regret minimization of $f_t(u_{t-H:t})$ can be done in the setting of OCO with memory. Lastly, we state the properties assumed for a controller $\mathcal{C}$.

\begin{assumption}\label{assmp:control}
    For a controller $\mathcal{C}$ with action set sequence $\mathcal{U}_{1:T}$, and policy class $\Pi$, assume
    \begin{enumerate}[(i)]
        \item $\mathcal{U}_{1:T}$ has $(H, \eps)$-bounded memory.
        \item For all $t \in [T]$, the proxy loss $f_t(u_{t-H:t}) = c_t(\hat{x}_t, u_t)$ is coordinate-wise $L$-Lipschitz.
        \item $\mathcal{C}$ attains policy regret $\reg_{\mathcal{C}}(T)$ with respect to $\Pi$, and action shift $\shift_{\mathcal{C}}(T)$.
    \end{enumerate}
\end{assumption}

The first two (i), (ii) points of the assumptions above concern the control setup only as they are properties of the action set sequence, system matrices, and loss functions but not the controller itself. The last (iii) point simply denotes the policy regret and action shift of the controller over time-varying dynamics. As shown later in section \ref{sec:apply_control}, Assumption \ref{assmp:control} is not vacuous given the previous results in control \cite{agarwal2019online}, \cite{simchowitz2020improper}, \cite{simchowitz2020making}.

\ignore{
\begin{claim}\label{claim:appl}
Let $\mathcal{C}_{\text{GFC}}$ be the GFC control algorithm \citep{simchowitz2020improper}, with $\mathcal{U}_{1:T}$ action set sequence and policy class $\Pi$ of strongly stable linear controllers. This setup satisfies the first two properties of Assumption \ref{assmp:control} with $H = \O(\log(1/\eps))$ and $L = \O(\sqrt{H})$. Furthermore, on a fixed LDS, i.e. $(A_t, B_t) = (A, B), \forall t \in [T]$, the controller $\mathcal{C}_{\text{GFC}}$ attains policy regret $\reg_{\C_{\text{GFC}}}(T) = \Theta(\text{poly}(\log T))$ with respect to $\Pi$ and action shift $\shift_{\C_{\text{GFC}}}(T) = \Theta(\text{poly}(\log T))$.
\end{claim}
}

\pg{say we assume noises bounded by $1$ for simplicity, say smth about bound on $A$, $B$ too}
